# Supplementary material for: Predicting Livelihood Indicators from Community-Generated Street-Level Imagery
Source: arXiv:2006.08661 source file (2021-02-26)
Supplement: Supplementary file 1 [file appendix.tex]

\section{Appendix}\label{appendix}

We first show tree visualizations for each indicator in India and Kenya. Then, we visualize the output predictions of the Obj-Clusterwise model by indicator in either country.

% \paragraph{Ablation Analysis} 
% In order to verify the importance of certain features, we conducted ablation studies by training the Random Forest regressor on all features and eliminating the top three most important ones at test time. $r^2$ dropped from 0.52 to 0.10 for poverty, from 0.85 to 0.73 for population density, and from 0.54 to -0.36 for women's BMI \dl{is this negative correct?}\jl{Yes, we got a negative r2 here}. Classification accuracy was less affected, dropping by 1.5\% for poverty (5.57\% with the GBDT), 5.01\% for population density (GBDT 9.36\%), and 4.65\% for BMI (GBDT 7.43\%). This is likely because the classification task requires less precision, and the model can depend on other salient features. It also demonstrates how the presence and magnitude of features can be very useful for finer grained predictions for regression. \burak{Can you just add a bar plot like Kumar did? It is hard to see the effect in the text.}

\subsection{Visualizations of Decision Trees}

We train a 100\% Pooled decision tree classifier and regressor with a max depth of 3 to predict poverty in India and Kenya. We then use the visualization tool presented by \cite{ParrTree} to visualize the tree. Each node displays the object class name and threshold that determines how to split the node (left child means $<$ the threshold, right child $\geq$ the threshold). Leaves represent predictions, where $n$ is the number of clusters assigned to that leaf.

For the classification trees, the histograms show the feature space distribution for a single feature, with the colors indicating the relationship between feature space and target class. For example, for the "car" histogram in Figure \ref{fig:iapovtrees}, we see that the yellow bars are clustered at the lower end, which is intuitive for low wealth. The histogram gets proportionally shorter as the number of clusters that reach the node decreases, and the leaf size becomes smaller as well. \protect\cite{ParrTree} motivates the use of pie charts to show quickly an indication of the strong majority category through color and size of slice.

For the regressor, feature-target space is shown with a scatterplot of feature vs. target. Regressor leaves use a strip plot to show the distribution explicitly (the number of dots is number of clusters assigned to the leaf), and the leaf prediction is the distribution center of mass, or mean, which is denoted with a dashed line.

\begin{figure}[!h]
\centering
\begin{subfigure}{\linewidth}
\includegraphics[width=\linewidth]{images/trees/pov_label_tree_fancy_short.png}\\
\includegraphics[width=\linewidth]{images/trees/pov_tree_fancy_short.png}
 \caption{India. Classification on top, regression on bottom.
 }
 \label{fig:iapovtrees}
\end{subfigure}

\begin{subfigure}{\linewidth}
\includegraphics[width=\linewidth]{images/trees/ke_pov_label.pdf}\\
\includegraphics[width=\linewidth]{images/trees/ke_pov_tree.pdf}
 \caption{Kenya. Classification on top, regression on bottom.
 }
 \label{fig:povtrees}
 \end{subfigure}
\caption{Decision tree visualization for wealth prediction. Recall that we consider poverty to be the inverse of wealth. Classification on top, regression on bottom.
 }
\end{figure}

\begin{figure}[!h]
\centering
    \begin{subfigure}{\linewidth}
    \includegraphics[width=\linewidth]{images/trees/pop_label_tree_fancy.pdf}\\
    \includegraphics[width=\linewidth]{images/trees/pop_tree_fancy.png}
     \caption{India. Classification on top, regression on bottom.
     }
     \end{subfigure}
     \label{fig:iapoptrees}
 
    \begin{subfigure}{\linewidth}
    \includegraphics[width=\linewidth]{images/trees/ke_pop_label.pdf}\\
    \includegraphics[width=\linewidth]{images/trees/ke_pop_tree.pdf}
     \caption{Kenya. Classification on top, regression on bottom.
     }
    \end{subfigure}
    \label{fig:kepoptrees}
    \caption{Decision tree visualization for population density prediction. Classification on top, regression on bottom.
    }
\end{figure}

\begin{figure}[!h]
\centering
\includegraphics[width=\linewidth]{images/trees/bmi_label_tree_fancy.pdf}\\
\includegraphics[width=\linewidth]{images/trees/bmi_tree_fancy.png}
 \caption{Decision tree visualization for women's BMI prediction in India. Note that women's BMI data was not available in the 2014 Kenya DHS survey. Classification on top, regression on bottom. 
 }
 \label{fig:bmitrees}
\end{figure}

\FloatBarrier
\clearpage
\subsection{Visualizations of Predictions}
Here we map our classification predictions across the country using the \textbf{Obj-Clusterwise} model. Correct predictions are green. False positives (predicted as "high" area for indicator but actually "low") are marked in red, while false negatives (predicted as "low" but actually "high") are colored purple.

\begin{figure}[!h]
\centering
\includegraphics[width=0.8\linewidth]{images/maps/Poverty_Label_Truth-Predictions_Diff.png}
    \caption{India - Map of poverty classification predictions.}
\label{fig:iapovmap}
\end{figure}

\begin{figure}[!h]
\centering
\includegraphics[width=0.7\linewidth]{images/maps/ke_pov_diff.pdf}
    \caption{Kenya - Map of poverty classification predictions.}
\label{fig:kepovmap}
\end{figure}

\begin{figure}[!h]
\centering
    \includegraphics[width=0.8\linewidth]{images/maps/Population_Label_Truth-Predictions_Diff.png}
    \caption{India - Map of population density classification predictions.}
\label{fig:iapopmap}
\end{figure}

\begin{figure}[!h]
\centering
\includegraphics[width=0.8\linewidth]{images/maps/ke_pop_diff.pdf}
    \caption{Kenya - Map of population density classification predictions.}
\label{fig:kepopmap}
\end{figure}

\begin{figure}[!h]
\centering
    \includegraphics[width=0.8\linewidth]{images/maps/BMI_Label_Truth-Predictions_Diff.png}
    \caption{India - Map of predictions for women's BMI classification predictions.}
\label{fig:bmimap}
\end{figure}
